# Supplementary material for: Radiative type-I seesaw neutrino masses
Source: arXiv:1910.04178 source file (2019-10-09)
Supplement: Supplementary file 1 [file 5-Appendix.tex]

\section{Appendix} \label{sec:appendix}

\subsection{More options}
\subsubsection{Option 2}

\begin{table}[h!]
\begin{center}
\begin{tabular}{| c || c | c || c |}
  \hline
  \hspace{0.1cm} Fields \hspace{0.1cm}  &  $SU(3)_C \times SU(2)_L \times U(1)_Y$  &  \hspace{0.2cm} $Z_4$ \hspace{0.2cm}  &  Residual $Z_2$  \\
\hline \hline
                   $L$ & ($\mathbf{1}$, $\mathbf{2}$, -1/2) &  $1$ &  $1$ \\
                 $e^c$ & ($\mathbf{1}$, $\mathbf{1}$,    1) &  $1$ &  $1$ \\
               $\nu_R$ & ($\mathbf{1}$, $\mathbf{1}$,    0) & $-1$ &  $1$ \\
                   $H$ & ($\mathbf{1}$, $\mathbf{2}$,  1/2) &  $1$ &  $1$ \\
\hline
  ($\chi_{L}$, $\chi_{R}$) & ($\mathbf{1}$, $\mathbf{1}$,    1) &   ($i$, $-i$) &  ($-1$, $-1$) \\
  ($\psi_{L}$, $\psi_{R}$) & ($\mathbf{1}$, $\mathbf{2}$,  1/2) &  ($-i$, $-i$) &  ($-1$, $-1$) \\
                    $\eta$ & ($\mathbf{1}$, $\mathbf{2}$,  1/2) &           $i$ &          $-1$ \\
    \hline
  \end{tabular}
\end{center}
\caption{Particle content of the example model that generates the one-loop diagram of \fig{fig:model 1-2} once the $Z_4$ is softly broken by the vector-like mass term $\bar \chi_R \chi_L$. After the breaking of $Z_4$ a remnant $Z_2$ is conserved.}
 \label{tab:fields}
\end{table}%

\begin{figure}[h!]
    \centering
    \begin{tikzpicture}[line width=1. pt, scale=1.5]
    % FERMIONS %
        \draw[fermion] (-1.5,0) -- (-1,0)
            node[midway, below] {$L_\alpha$};
        \draw[fermionbar] (-1,0) -- (-0.5,0)
            node[midway, below] {$\chi_L$};
        \draw[fermion] (-0.5,0) -- (0,0)
            node[midway, below] {$\bar \chi_R$};
        \draw[fermionbar] (0,0) -- (0.5,0)
            node[midway, below] {$\psi_L$};
        \draw[fermion] (0.5,0) -- (1,0)
            node[midway, below] {$\bar \psi_R$};
        \draw[fermion] (1,0) -- (1.5,0)
            node[midway, below] {$\nu_{R\beta}$};
    % SCALARS %        
        \draw[scalar] (-1,0) arc (180:0:1)
            node[midway,above] {$\eta$};
        \draw[scalarbar] (0,0) -- (0,-.5)
            node[below] {$H$};
            
        \node at (-0.5,0) {$\mathbf{\otimes}$};
        \node at (0.5,0) {$\mathbf{\times}$};
    \end{tikzpicture}
    \caption{One-loop Dirac neutrino mass term. The diagram is realized when the $Z_4$ is softly broken (denoted by the symbol $\otimes$). As the symmetry is broken in two units, the diagram is still invariant under a remnant $Z_2$ of $Z_4$.}
    \label{fig:model 1-2}
\end{figure}

The Dirac mass term can be computed directly from the diagram of \fig{fig:model 1-2} given the Lagrangian \eqref{eq:lag 1-2} in the mass insertion approximation. For simplicity, the vector-like masses of the internal fermions are set to $M_F$.
\begin{equation} %\label{eq:}
    m_D \approx \frac{1}{16\pi^2} v Y_L Y_X Y_R \; \mathcal{I}(m_S^2/M_F^2),
\end{equation}
where the flavour indices have been omitted form the Yukawas and the loop integral $\mathcal{I}(x)$ can be written in terms of the Passarino-Veltman $B_0$ function \cite{Passarino:1978jh} as,
\begin{equation} %\label{eq:}
    \mathcal{I}(x) = \frac{1}{1-x} \left[ B_0(0,1,1) - B_0(0,1,x) \right].
\end{equation}

\begin{figure}[h!]
    \centering
    \includegraphics[width=0.7\textwidth]{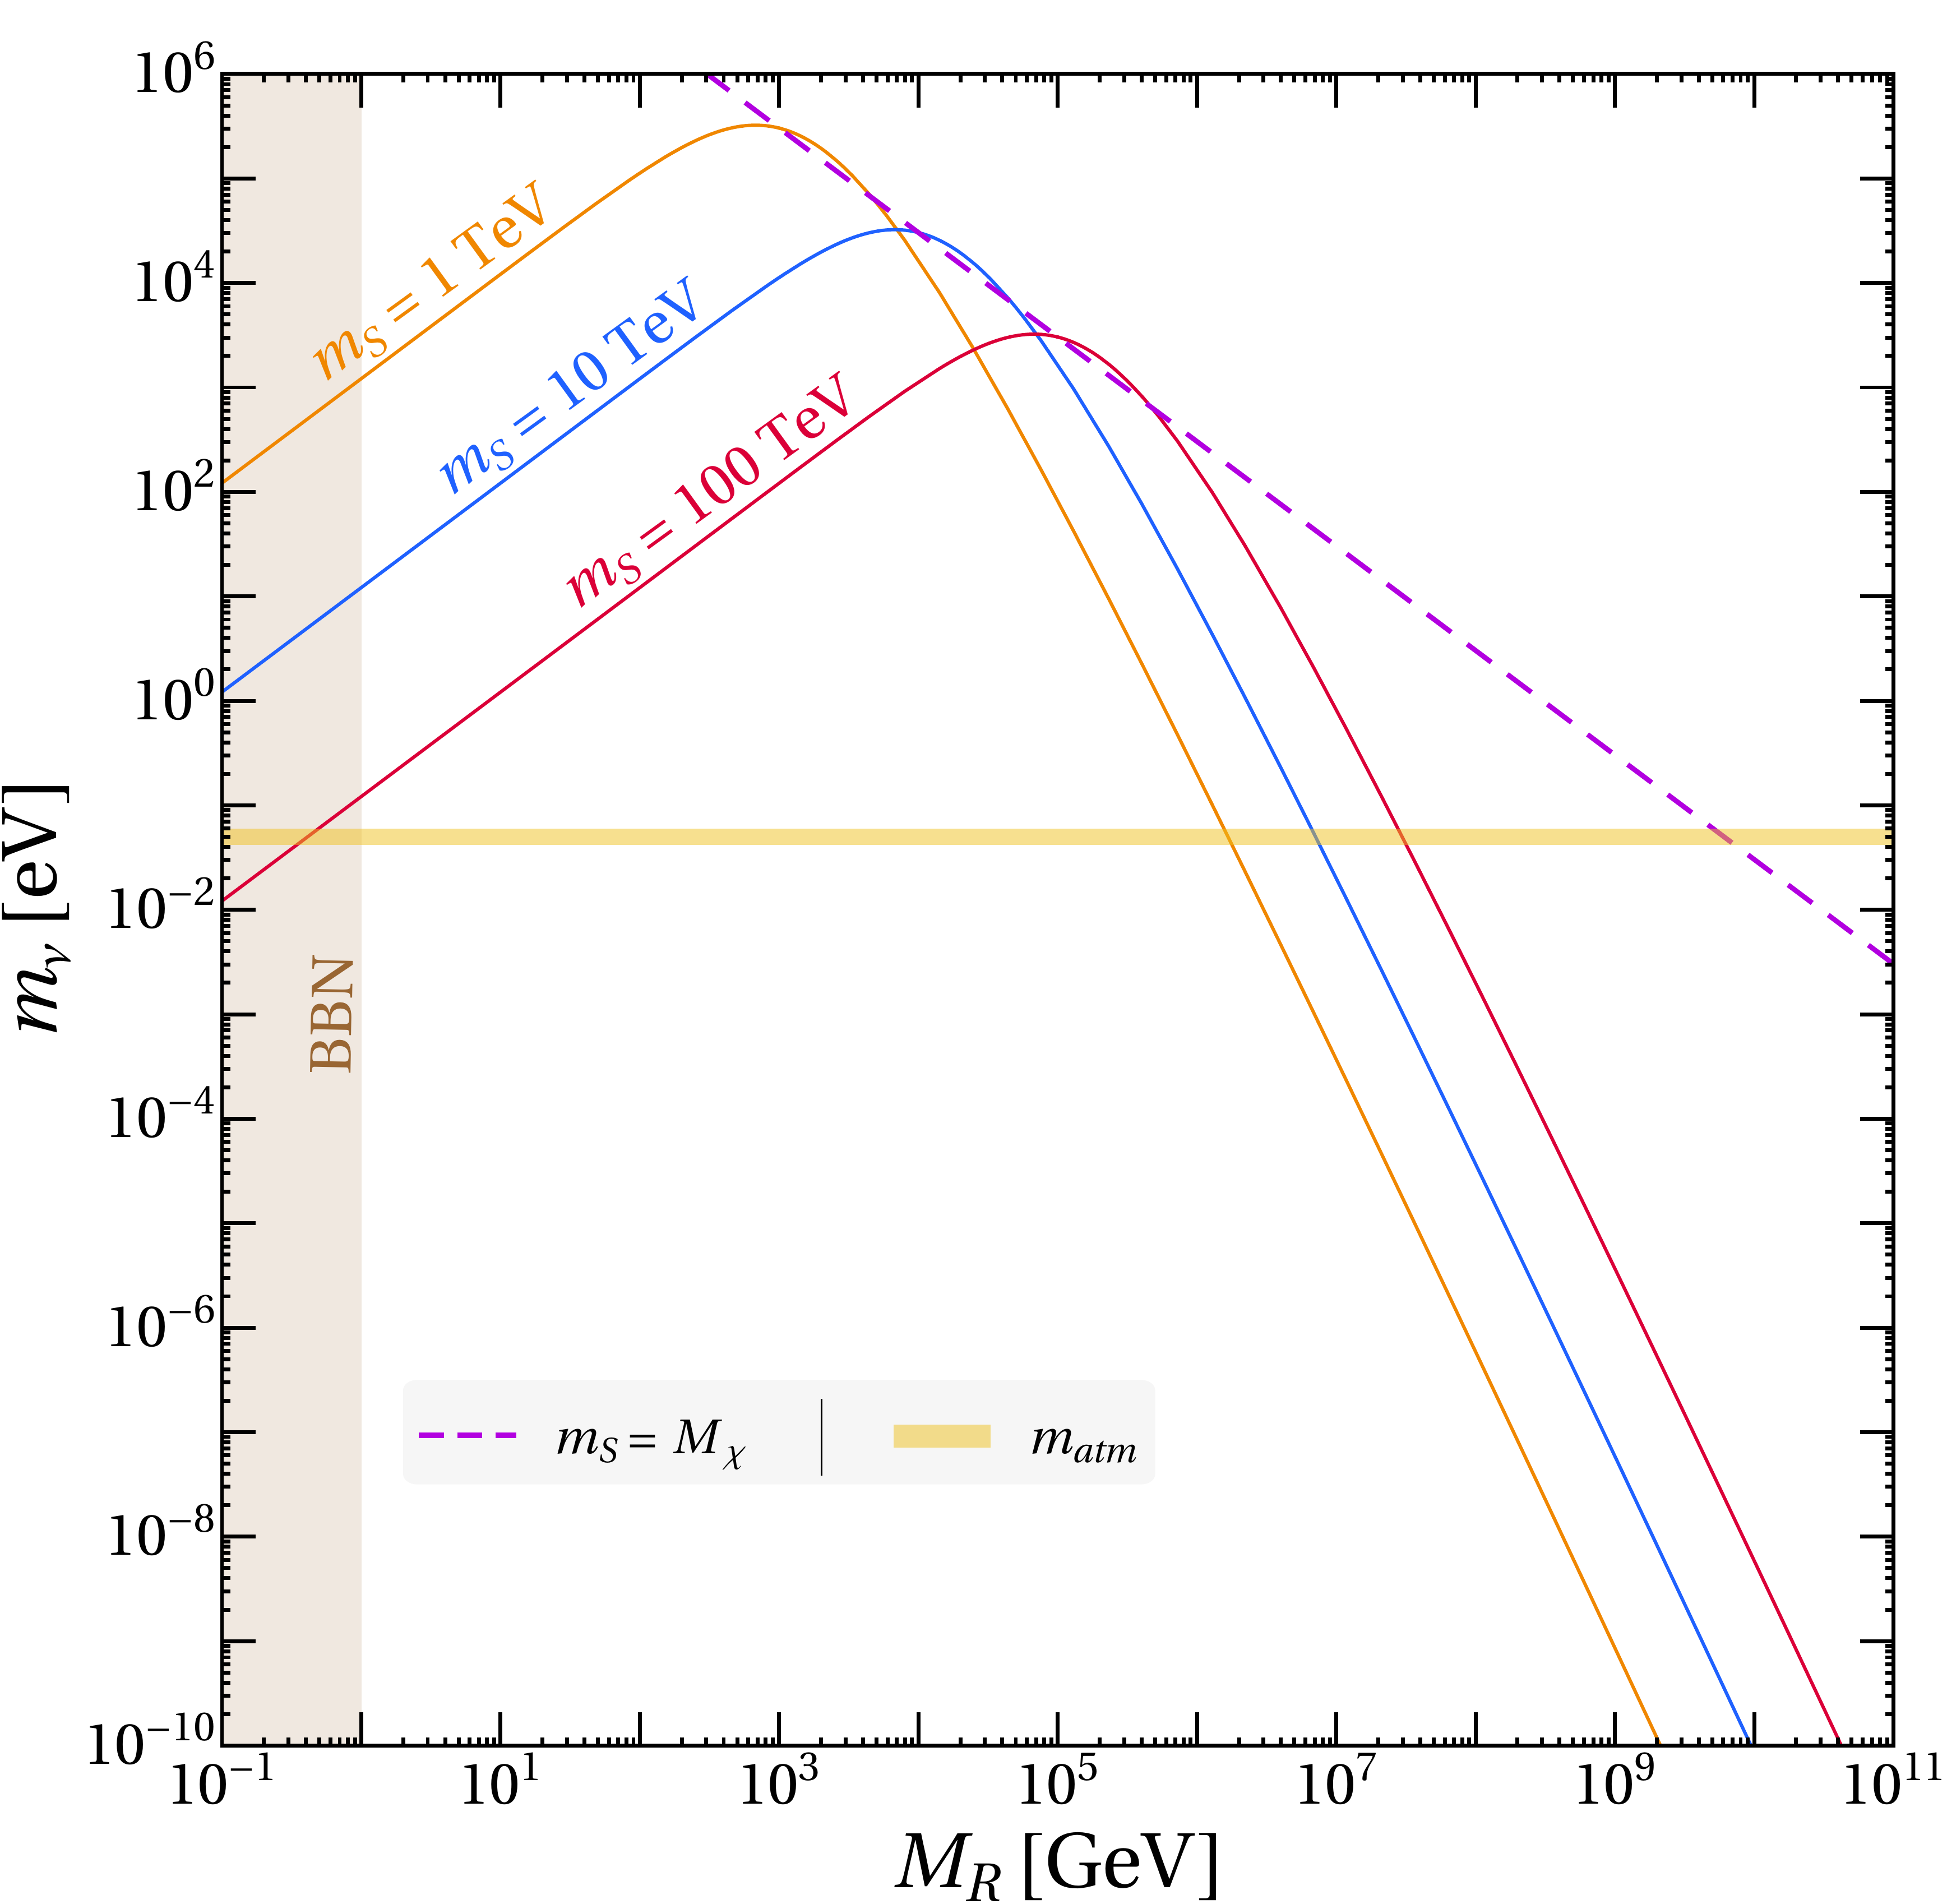}
    \caption{caption}
    \label{fig:mass plot 1-2}
\end{figure}

\subsection{Estimations}

\noindent Two loop:

\begin{figure}[h!]
    \centering
    \includegraphics[width=0.7\textwidth]{Figures/mass_plot_2loop}
    \caption{Two-loop neutrino mass scale for different choices of the scalar masses. Calculation made using the estimated neutrino approximation.}
    \label{fig:mass plot 2}
\end{figure}
